# Supplementary material for: Towards rational design of power-law rheology via DNA nanostar networks
Source: arXiv:2308.14699 source file (2023-08-28)
Supplement: Supplementary file 1 [file Supp_Info.pdf]

# Supplementary materials for Towards rational design of power-law rheology via DNA nanostar networks

Nathaniel Conrad

*Department of Physics, University of California, Santa Barbara, CA 93106\**

Omar A. Saleh

*Department of Physics, University of California, Santa Barbara, CA 93106\* and*

*Materials Department, University of California, Santa Barbara, CA 93106*

Deborah K. Fygenson

*Department of Physics, University of California, Santa Barbara, CA 93106\* and*

*Department of Biomolecular Science and Engineering,*

*University of California, Santa Barbara, CA 93106<sup>†</sup>*

(Dated: July 28, 2023)

- 
- [1] S. C. Grindy, R. Learsch, D. Mozhdehi, J. Cheng, D. G. Barrett, Z. Guan, P. B. Messersmith, and N. Holten-Andersen, Control of hierarchical polymer mechanics with bioinspired metal-coordination dynamics, *Nature Materials* **14**, 1210 (2015).
  - [2] A. Takeh and S. Shanbhag, A computer program to extract the continuous and discrete relaxation spectra from dynamic viscoelastic measurements, *Applied Rheology* **23**, 24628 (2013).

---

\* Currently at McKetta Department of Chemical Engineering, The University of Texas at Austin, Austin, TX 78712

<sup>†</sup> Corresponding authors' e-mail: nconrad@utexas.edu, fygenson@ucsb.edu, saleh@ucsb.edu

| Name                  | Sequence (5'→3')                                    | Extinction Coefficient<br>(L/(mol cm)) |
|-----------------------|-----------------------------------------------------|----------------------------------------|
| V1 $\gamma_4$         | CTACTATGGCGGGTGATAAAAGGGAAGAGCATGCCCATCCATGCGCGCA   | 480700                                 |
| V2 $\gamma_4$         | GGATGGGCATGCTCTTCCCAATCAACTGCCTGGTGATACGATGCGCGCA   | 457600                                 |
| V3 $\gamma_4$         | CGTATCACCAGGCAGTTGAAAATGCGAGGGTCCAATACCGATGCGCGCA   | 479800                                 |
| S4 $\gamma_4$         | CGGTATTGGACCCTCGCATAAATTATCACCCGCCATAGTAGATGCGCGCA  | 467000                                 |
| V1 $\alpha_6$         | CTACTATGGCGGGTGATAAAACGGGAAGAGCATGCCCATCCACGATCG    | 484100                                 |
| V2 $\alpha_6$         | GGATGGGCATGCTCTTCCCGAATCAACTGCCTGGTGATACGACGATCG    | 458900                                 |
| V3 $\alpha_6$         | CGTATCACCAGGCAGTTGAGAACATGCGAGGGTCCAATACCGACGATCG   | 483300                                 |
| V4 $\alpha_6$         | CGGTATTGGACCCTCGCATGAACCATGCTGGACTCAACTGACACGATCG   | 462500                                 |
| V5 $\alpha_6$         | GTCAGTTGAGTCCAGCATGGAACGCATCAGTTGCGGCGCCGACGATCG    | 465500                                 |
| S6 $\alpha_6$         | GCGGCGCCGCAACTGATGCGAATTTATCACCCGCCATAGTAGACGATCG   | 467200                                 |
| V1 $\alpha_3\gamma_3$ | CTACTATGGCGGGTGATAAAACGGGAAGAGCATGCCCATCCACGATCG    | 472100                                 |
| V2 $\alpha_3\gamma_3$ | GGATGGGCATGCTCTTCCCGAATCAACTGCCTGGTGATACGATGCGCGCA  | 468100                                 |
| V3 $\alpha_3\gamma_3$ | CGTATCACCAGGCAGTTGAAACATGCGAGGGTCCAATACCGACGATCG    | 472000                                 |
| V4 $\alpha_3\gamma_3$ | CGGTATTGGACCCTCGCATGAACATGCTGGACTCAACTGACATGCGCGCA  | 470700                                 |
| V5 $\alpha_3\gamma_3$ | GTCAGTTGAGTCCAGCATGAACGCATCAGTTGCGGCGCCGACGATCG     | 455400                                 |
| S6 $\alpha_3\gamma_3$ | GCGGCGCCGCAACTGATGCGAATTTATCACCCGCCATAGTAGATGCGCGCA | 474500                                 |
| V1X $\gamma_3$        | CTACTATGGCGGGTGATAAAACGGGAAGAGCATGCCCATCC           | 402700                                 |
| V2 $\alpha_3X_3$      | GGATGGGCATGCTCTTCCCGAATCAACTGCCTGGTGATACG           | 383400                                 |
| V3X $\gamma_3$        | CGTATCACCAGGCAGTTGAAACATGCGAGGGTCCAATACCG           | 402700                                 |
| V4 $\alpha_3X_3$      | CGGTATTGGACCCTCGCATGAACATGCTGGACTCAACTGAC           | 385900                                 |
| V5X $\gamma_3$        | GTCAGTTGAGTCCAGCATGAACGCATCAGTTGCGGCGCCG            | 386000                                 |
| S6 $\alpha_3X_3$      | GCGGCGCCGCAACTGATGCGAATTTATCACCCGCCATAGTAG          | 389800                                 |
| V1 $\alpha_3\gamma_2$ | CTACTATGGCGGGTGATAAAACGGGAAGAGCATGCCCATCCACGATCG    | 484100                                 |
| V2 $\alpha_3\gamma_2$ | GGATGGGCATGCTCTTCCCGAATCAACTGCCTGGTGATACGATGCGCGCA  | 468100                                 |
| V3 $\alpha_3\gamma_2$ | CGTATCACCAGGCAGTTGAAACATGCGAGGGTCCAATACCGACGATCG    | 472000                                 |
| V4 $\alpha_3\gamma_2$ | CGGTATTGGACCCTCGCATGAACATGCTGGACTCAACTGACATGCGCGCA  | 470700                                 |
| S5 $\alpha_3\gamma_2$ | GTCAGTTGAGTCCAGCATGAATTTATCACCCGCCATAGTAGACGATCG    | 469700                                 |
| V1 $\alpha_4\gamma_2$ | CTACTATGGCGGGTGATAAAAGGGAAGAGCATGCCCATCCATGCGCGCA   | 492700                                 |
| V2 $\alpha_4\gamma_2$ | GGATGGGCATGCTCTTCCCAACTCAACTGCCTGGTGATACGACGATCG    | 448400                                 |
| V3 $\alpha_4\gamma_2$ | CGTATCACCAGGCAGTTGAGAACATGCGAGGGTCCAATACCGACGATCG   | 483300                                 |
| V4 $\alpha_4\gamma_2$ | CGGTATTGGACCCTCGCATGAACATGCTGGACTCAACTGACATGCGCGCA  | 470700                                 |
| V5 $\alpha_4\gamma_2$ | GTCAGTTGAGTCCAGCATGAACGCATCAGTTGCGGCGCCGACGATCG     | 455400                                 |
| S6 $\alpha_4\gamma_2$ | GCGGCGCCGCAACTGATGCGAATTTATCACCCGCCATAGTAGACGATCG   | 467200                                 |
| V1 $\alpha_4X_2$      | CTACTATGGCGGGTGATAAAAGGGAAGAGCATGCCCATCC            | 407900                                 |
| V2 $\alpha_4\gamma_2$ | GGATGGGCATGCTCTTCCCAACTCAACTGCCTGGTGATACGACGATCG    | 448400                                 |
| V3 $\alpha_4\gamma_2$ | CGTATCACCAGGCAGTTGAGAACATGCGAGGGTCCAATACCGACGATCG   | 483300                                 |
| V4 $\alpha_4X_2$      | CGGTATTGGACCCTCGCATGAACATGCTGGACTCAACTGAC           | 385900                                 |
| V5 $\alpha_4\gamma_2$ | GTCAGTTGAGTCCAGCATGAACGCATCAGTTGCGGCGCCGACGATCG     | 455400                                 |
| S6 $\alpha_4\gamma_2$ | GCGGCGCCGCAACTGATGCGAATTTATCACCCGCCATAGTAGACGATCG   | 467200                                 |
| V1 $\alpha_2\gamma_4$ | CTACTATGGCGGGTGATAAAAGGGAAGAGCATGCCCATCCATGCGCGCA   | 492700                                 |
| V2 $\alpha_2\gamma_4$ | GGATGGGCATGCTCTTCCCAATCAACTGCCTGGTGATACGATGCGCGCA   | 457600                                 |
| V3 $\alpha_2\gamma_4$ | CGTATCACCAGGCAGTTGAAACATGCGAGGGTCCAATACCGACGATCG    | 472000                                 |
| V4 $\alpha_2\gamma_4$ | CGGTATTGGACCCTCGCATGAACATGCTGGACTCAACTGACATGCGCGCA  | 470700                                 |
| V5 $\alpha_2\gamma_4$ | GTCAGTTGAGTCCAGCATGAACGCATCAGTTGCGGCGCCGATGCGCGCA   | 464600                                 |
| S6 $\alpha_2\gamma_4$ | GCGGCGCCGCAACTGATGCGAATTTATCACCCGCCATAGTAGACGATCG   | 457000                                 |

FIG. 1. Sequences of DNA strands used to assemble the various DNA nanostars of this study.

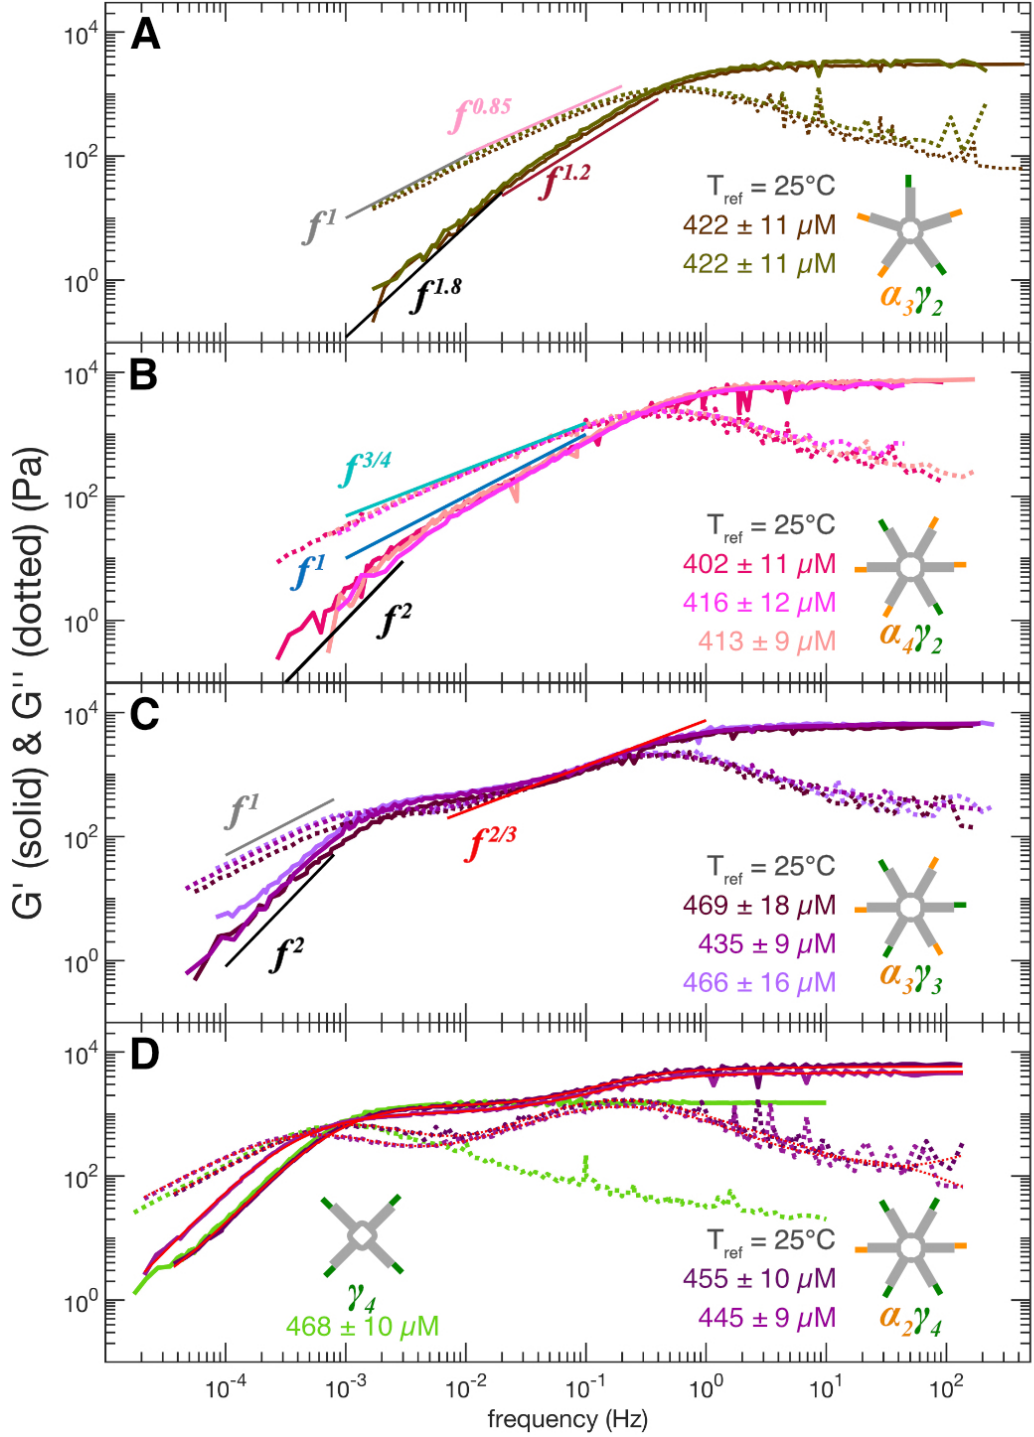

FIG. 2. Measured storage and loss moduli versus frequency of (A)  $\alpha_3\gamma_2$ , (B)  $\alpha_4\gamma_2$ , (C)  $\alpha_3\gamma_3$ , and (D)  $\alpha_2\gamma_4$  NSs measured at 1% strain and a reference temperature of  $25^\circ\text{C}$ . In (D),  $\gamma_4$  is also plotted to demonstrate the overlap with the  $\alpha_2\gamma_4$  at the lowest frequencies. All solutions were hydrated in a tris-HCl EDTA buffer solution (40 mM Tris, 11.5 mM HCl, and 1 mM EDTA) with an added salt concentration of 300 mM NaCl.

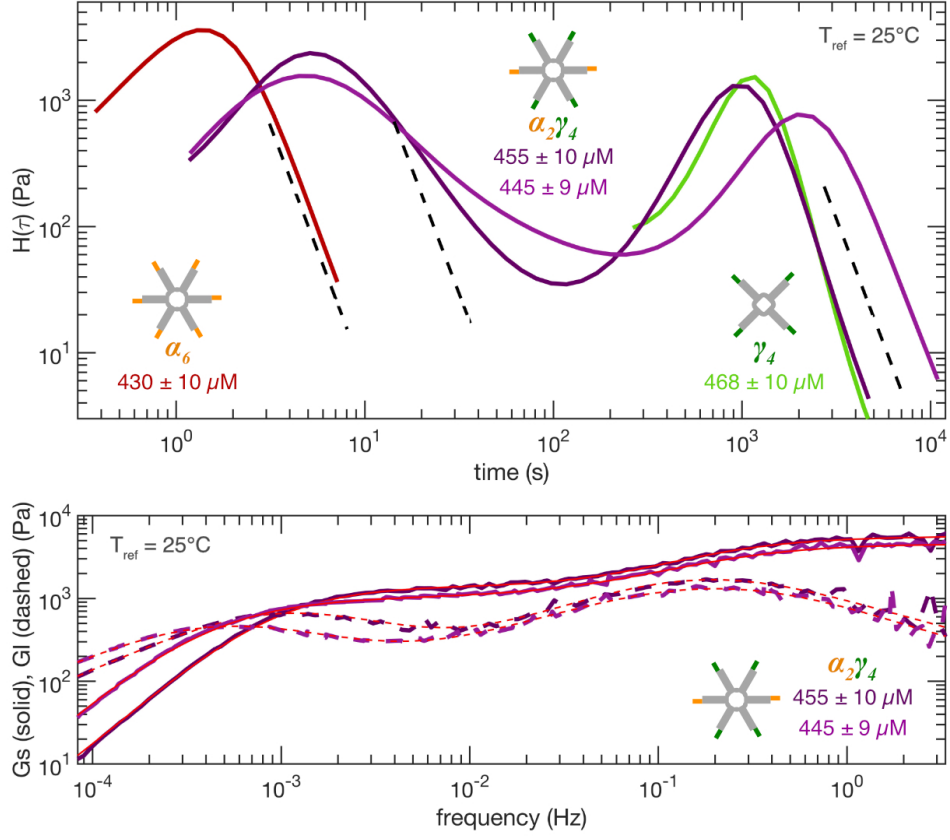

FIG. 3. **(Top panel)** Relaxation spectrum,  $H(\tau)$ , versus time for  $\gamma_4$  (green),  $\alpha_6$  (red), and  $\alpha_2\gamma_4$  (purple hues) NS solutions. The dashed lines are guides for the eye to show how the trailing slope of the single mode in the  $\gamma_4$  and  $\alpha_6$  NS spectra decreases with time. The observed difference in trailing slope of the single mode homotypic NS spectrum and shortest-lived mode of the heterotypic  $\alpha_2\gamma_4$  spectrum indicates there are additional modes not present in the homotypic NS solutions [1]. Consequently, the  $\alpha_2\gamma_4$  NS solutions are not purely bi-modal Maxwell materials, despite having two distinct peaks in their relaxation spectrum. **(Bottom panel)** Plot of  $G'$  and  $G''$  versus frequency of concentrated solutions of the corresponding  $\alpha_2\gamma_4$  NSs at 1% strain and a reference temperature of  $25^\circ\text{C}$ . The red lines are generalized Maxwell model fits to the measured  $G'$  and  $G''$  versus frequency. The fits are then used to extract the corresponding  $H(\tau)$  shown in the top panel. The code used to extract  $H(\tau)$  was made by Arsia Takeh and Sachin Shanbhag [2] and available at <https://www.mathworks.com/matlabcentral/fileexchange/40458-respect>.
